# Supplementary material for: SWE-Together: Evaluating Coding Agents in Interactive User Sessions
Source: arXiv:2606.29957 source file (2026-06-29)
Supplement: Supplementary file 1 [file appendix.tex]

\section{Simulator Action Distribution}
\label{app:action-distribution}

Table~\ref{tab:action-distribution} summarizes message-bearing simulator
actions across the 92-task $\times$ 5-agent interaction-analysis set
($2{,}459$ messages). These action counts describe what kinds of interventions
the simulator emits; the main paper uses User Correction, rather than a separate
action-weighted aggregate, as the model-facing interaction diagnostic.

\begin{table}[h]
\centering
\small
\begin{tabular}{lrrl}
\toprule
Action & $n$ & Mean / Med.\ words & Role in interaction \\
\midrule
\texttt{redirect}         & 1{,}213 & 21.6 / 17 & corrective feedback \\
\texttt{new\_requirement} &   685 & 20.4 / 11 & follow-up requirement \\
\texttt{question}         &   556 & 13.8 / 10 & clarification or verification \\
\texttt{check\_external}  &     5 & 15.8 / 14 & external-artifact request \\
\midrule
Total                     & 2{,}459 & --- & --- \\
\bottomrule
\end{tabular}
\caption{Per-action statistics for message-bearing simulator interventions.
These counts are descriptive and are not used as a model-ranking metric.}
\label{tab:action-distribution}
\end{table}

\paragraph{Relationship to User Correction.}
The action labels above describe the simulator's decision type, while User
Correction is computed from a separate multi-label annotation of message
content. This distinction matters because a single message may both introduce a
new requirement and correct an earlier mistake, or ask a question that functions
as a soft nudge. User Correction therefore counts explicit corrections and
nudges directly, rather than assigning fixed weights to simulator action names.

\paragraph{Examples.}
The qualitative differences are visible in representative turns from the pool:

\smallskip
\noindent\textit{\texttt{redirect}~--- read, diagnose, redirect:}
\begin{itemize}\itemsep2pt
  \item \emph{``that looks good but can you only show the times that actually have entries''}
  \item \emph{``Read the external configuration and the relevant implementation. Shouldn't the context window be smaller?''}
  \item \emph{``wait, that changes the numerical behavior instead of just fixing the build error. is there another way to fix it without changing the math?''}
\end{itemize}

\smallskip
\noindent\textit{\texttt{new\_requirement}~--- chain a follow-up task:}
\begin{itemize}\itemsep2pt
  \item \emph{``Okay, now, that new option? Document it in the user-facing help text.''}
  \item \emph{``ok, add a changelog entry that this new integration is now available''}
  \item \emph{``commit and push, then we can talk about the next set of features''}
\end{itemize}

\smallskip
\noindent\textit{\texttt{question}~--- outsource the analysis:}
\begin{itemize}\itemsep2pt
  \item \emph{``Is this well structured? Will it do this in a nice way? Will it work well on mobile and other devices?''}
  \item \emph{``What's the difference between the two implementations?''}
  \item \emph{``Are there hard-coded Linux config and data file paths?''}
\end{itemize}

%%%%%%%%%APPENDIX%%%%%%%%%
